# Supplementary material for: Privacy-preserving Cross-domain Routing Optimization -- A Cryptographic Approach
Source: arXiv:1505.05960 source file (2015-05-22)
Supplement: Supplementary file 1 [file 9_appendix.tex]

\section{Appendix}

\begin{algorithm}[!ht]
\caption{Privacy-preserving Shortest Path Tree Protocol} \label{alg:baseline}
\begin{algorithmic}[1]
%\REQUIRE
%\ENSURE
\FORALL{domain $D_i$ except $D_s$}
	\FORALL{$v,v' \in S_i \wedge D_i \neq D_s$}
		\STATE $C_i$ computes $e(vv')=E(d(vv'))$ and sends it to $C_s$
	\ENDFOR
\ENDFOR
\FORALL{$v,v'$ that $v \in S_i \wedge v' \in S_j \wedge S_i \neq S_j \wedge v \sim v'$ or $v,v' \in D_s \wedge v \sim v'$
\COMMENT{the link $vv'$ is an inter-domain link or is an intra-domain link in $D_s$}
}
	\STATE $C_s$ computes $e(vv')=E(c(vv'))$
\ENDFOR
\FORALL{$v \in S \wedge v \neq v_s$}
	\STATE $C_s$ computes $\begin{cases}f(v)=E'(2) &  \\ g(v)=E(0) & \\ h(v)=E'(\phi) & \end{cases}$
\ENDFOR
\STATE For source node $v_s$, $C_s$ computes $\begin{cases}f(v_s)=E'(2^{-1}) &  \\ g(v_s)=E(0) & \\ h(v_s)=E'(\phi) & \end{cases}$
\FOR{$i=1$ \TO $|S|-1$ }
	\FORALL{$v \sim v' \wedge v,v' \in S$}
		\STATE $\alpha(vv')=SecIf_0[D'(f(v))==D'(f(v')),$ $E(c_{max}|S|+1), R(g(v)+g(v')+e(vv'))]$
	\ENDFOR
	\FORALL{$v \sim v' \wedge v,v' \in S$}
		\STATE $\begin{cases}
			f(v) = SecIf_1[X, T_1, R'(f(v))] & \\
			g(v) = SecIf_1[X, T_2, R(g(v))] & \\
			h(v) = SecIf_1[X, T_3, R'(h(v))] & \\
			f(v')= SecIf_1[X, T_4, R'(f(v')] & \\
			g(v')= SecIf_1[X, T_5, R(g(v'))] & \\
			h(v')= SecIf_1[X, T_6, R'(h(v'))] &
			\end{cases}$
			\\ where $X$ is the condition that the plaintext of  $\alpha(vv')$ is the smallest among all the $\alpha$ values and $T_1$ to $T_6$ are computed as below.
		\STATE $\begin{cases}
			T_1 = SecIf_2[Y,E'(2^{-1}), R'(f(v))] & \\
			T_2 = SecIf_2[Y,R(\alpha(vv'),R(g(v))] & \\
			T_3 = SecIf_2[Y,E'(v'),R'(h(v))] & \\
			T_4 = SecIf_2[Y,R'(f(v'),E'(2^{-1}))] & \\
			T_5 = SecIf_2[Y,R(g(v'),R(\alpha(vv'))] & \\
			T_6 = SecIf_2[Y,R'(h(v'),E'(v))] &
		\end{cases}$ \\
			where $Y$ is the condition that $D'(f(v))==2$.
	\ENDFOR
\ENDFOR
\end{algorithmic}
\end{algorithm}

Algorithm~\ref{alg:baseline} shows the details of our shortest path tree protocol in Section \ref{sec:tree}.

Algorithm~\ref{alg:path_establishment} presents the pseudocode of the path establishment protocol in Section \ref{sec:path}.

\begin{algorithm}[!ht]
\caption{Path Establishment Protocol} \label{alg:path_establishment}
\begin{algorithmic}[1]
\REQUIRE All significant nodes' $g$ and $h$;\\
		 Source node $v_s$ and destination node $v_t$;
\ENSURE The shortest path $P$ from $v_s$ to $v_t$
\STATE $C_s$ computes partial decryption $PD(g(v))$ and $PD'(h(v))$, and then  sends them to $C$, the controller of $v$.
\STATE $C$ partially decrypts $PD(g(v))$ and $PD'(h(v))$ and gets the plaintext of $g(v)$ and $h(v)$: $dg(v)$ and $dh(v)$.
\STATE $v_t=v_t$
\IF{$v_t \not \in S$}
	%\STATE Let $C_t$ be the controller of $v_t$
	%\STATE Let $D_t$ be the domain of $v_t$
	\STATE Let $S_t$ be the significant node set of $D_t$
	\STATE $v_{min}=-1,d_{min}=\infty$
	\FORALL{$v \in S_t$}
		\IF{$dg(v) + d(vv_t) < d_{min}$}
			\STATE $d_{min}=dg(v) + d(vv_t)$, $v_{min} = v$
		\ENDIF
	\ENDFOR
	\STATE Add the intra-domain path from $v_{min}$ to $v_t$ to $P$.% and set the forwarding table entries for $v_t$ according to the path.
	\STATE Let $v_t=v_{min}$
\ENDIF
\STATE Now we construct the path from $v_s$ to $v_t$.
\WHILE{$v_t \neq v_s$}
	\IF{$dh(v_t) \in S_t$
	\COMMENT{$dh(v_t) \sim v_t$ is an intra-domain link}
	}
		\STATE Add the intra-domain path from $dh(v_t)$ to $v_t$ to $P$.% and set the forwarding table entries for $v_t$ according to the path.
	\ENDIF
	\IF{$dh(v_t) \not \in S_t$
	\COMMENT{$dh(v_t) \sim v_t$ is an inter-domain link}
	}
		\STATE Add $dh(v_t) \sim v_t$ to $P$.% and let the controller of $dh(v_t)$ set the forwarding table entry $T(dh(v_t))[v_t]=v_t$.
	\ENDIF
	\STATE Let $v_t=dh(v_t)$
\ENDWHILE
\end{algorithmic}
\end{algorithm}

The algorithm of  optimized PSPT construction is presented in Algorithm~\ref{alg:optimal}. The result of the optimized protocol is that every controller gets the struct of the shortest path tree $T$, which includes whole shortest path tree information. The struct $T$ has members $T[v].f$, $T[v].g$ and $T[v].h$: $T[v].f$ is a bool value indicating whether node $v$ is in $T$; $T[v].g$ is a plaintext indicating the distance from $v_s$ to $v$; $T[v].h$ is a plaintext indicating the parent node of $v$. And in the algorithm we assume that the number of domain is $n$ and the shortest path tree of each domain is $T_i$. With $T_i(i =1,2,\ldots,n)$, $C_i$ can easily get the shortest path from $v_s$ to $v_t$ using Algorithm~\ref{alg:path_establishment}.

%The formal description of the optimized protocol can be found in Algorithm~\ref{alg:optimal}.

\begin{algorithm}[!ht]
\caption{Optimized PSPT Construction Protocol} \label{alg:optimal}
\begin{algorithmic}[1]
%\REQUIRE
\ENSURE the shortest path tree $T_i$ of each domain
\FOR{$i = 1$ \TO $n$}
	\STATE $C_i$ does $T_i[v_s].f=true$, $T_i[v_s].g=0$, $T_i[v_s].h=v_s$
\ENDFOR
\FOR{$k = 1$ \TO $|S|-1$}
	\FOR{$i = 1$ \TO $n$}
		\STATE Domain $i$ does the following things.
		\STATE $v_{i}=-1$, $d_{i}=\infty$, $h_{i}=-1$
		\FORALL{$v \in S_i$}
			\FORALL{$v'$ s.t. $T_i[v']==true$}
				\IF{$d > T_i[v'].g+d(v'v)$}
					\STATE $d = T_i[v'].g+d(v'v)$
				\ENDIF
			\ENDFOR
			\IF{$d_{i} > d$}
				\STATE $d_{i}=d$, $v_{i}=v$, $h_{i}=v'$
			\ENDIF
		\ENDFOR
		\STATE $D_i$ keeps $<v_{i},d_{i},h_{i}>$ as its candidate node's information
	\ENDFOR
	\STATE $c_{min}=1$
	\FOR{$i = 2$ \TO $n$}
		\STATE $C_s$ send a message to $C_{c_{min}}$ and $C_i$ to let them run the DGK protocol.
		\STATE Upon receiving the message, $C_{c_{min}}$ and $C_i$ run DGK protocol to compare $d_{c_{min}}$ and $d_i$. The result of the comparison is sent to $C_s$.
		\IF{$d_{i} < d_{c_{min}}$}
			\STATE $C_s$ does $c_{min}=i$
		\ENDIF
	\ENDFOR
	\STATE $C_{c_{min}}$ broadcast $<v_{c_{min}},d_{c_{min}},h_{c_{min}}>$.
	\FOR{$i = 1$ \TO $n$}
		\STATE $C_i$ receives $<v_{c_{min}},d_{c_{min}},h_{c_{min}}>$ from $C_{c_{min}}$\COMMENT{except $C_{c_{min}}$ itself}
		\STATE $C_i$ does $T_i[v_{c_{min}}].f=true$, $T_i[v_{c_{min}}].g=d_{c_{min}}$, $T_i[v_{c_{min}}].h=h_{c_{min}}$
	\ENDFOR
\ENDFOR
\end{algorithmic}
\end{algorithm}

The details of the bandwidth allocation protocol can be found in Alogirthm~\ref{alg:ba}.
\begin{algorithm}
\caption{Bandwidth Allocation Protocol} \label{alg:ba}
\begin{algorithmic}[1]
\REQUIRE the bandwidth demand $q$;
\ENSURE the path set $SP$ whose element is $<P, b_P>$ where $P$ is the path and $b_P$ is the bandwidth of $P$.
\STATE $b_t = 0$, $SP=\emptyset$
\WHILE{$b_t<q$}
	\STATE Run the shortest path tree protocol and path establishment protocol to get the path from $v_s$ to $v_t$, say, $P$.
	\FOR{$i=1$ \TO $n$}
		\STATE $b_i = \infty$
		\FORALL{$v \sim v' \in D_i \wedge v\sim v' \in P$}
			\IF{$b_i > b(v,v')$}
				\STATE $b_i = b(v,v')$
			\ENDIF
		\ENDFOR
	\ENDFOR	
	\STATE $c_{min}=1$
	\FOR{$i = 2$ \TO $n$}
		\STATE $C_s$ send a message to $C_{c_{min}}$ and $C_i$ to let them run the DGK protocol.
		\STATE Upon receiving the message, $C_{c_{min}}$ and $C_i$ run DGK protocol to compare $b_{c_{min}}$ and $b_i$. The result of the comparison is sent to $C_s$.
		\IF{$b_{i} < b_{c_{min}}$}
			\STATE $C_s$ does $c_{min}=i$
		\ENDIF
	\ENDFOR	
	\STATE $b_t = b_t + b_{c_{min}}$
	\FORALL{$v \sim v' \in P$}
		\STATE $b(v,v')=b(v,v')-b_{c_{min}}$
	\ENDFOR
	\STATE $BP = BP \cup \{<P, b_{c_{min}}>\}$
\ENDWHILE
\end{algorithmic}
\end{algorithm}
